# Supplementary material for: Thermodynamic formalism for subsystems of expanding Thurston maps II
Source: arXiv:2404.07247 source file (2024-04-10)
Supplement: Supplementary file 1 [file Pressure.tex]

\section{Pressures}
\label{sec:Pressures}
% For an expanding Thurston map $f \: S^2 \mapping S^2$ and a continuous function $\varphi \in C(S^2)$, we denote the topological pressure of $f$ with respect to $\varphi$ by $P(f, \varphi)$. 

In this subsection we are going to prove the following characterization of the topological pressure $P(f, \phi)$ of an expanding Thurston map $f$ with respect to a \holder continuous potential $\phi$.
\begin{proposition}    \label{prop:pressures with respect to tiles}
	Let $f$, $\mathcal{C}$, and $\phi$ satisfy the Assumptions in Section~\ref{sec:The Assumptions}. Then we have
	\begin{equation}    \label{eq:pressures with respect to tiles}
 		P(f, \phi) = \lim_{n \to +\infty} \frac{1}{n} \log \!\sum_{X^n \in \mathbf{X}^{n}(f,\, \mathcal{C}) } \exp \!\bigl(\! \sup \bigl\{ S_n \phi(x) \describe x \in X^n \bigr\} \bigr).
	\end{equation}
\end{proposition}

The key ingredients of the proof of Proposition~\ref{prop:pressures with respect to tiles} are distortion lemmas and the following characterization of the topological pressure $P(f, \phi)$ established in \cite[Proposition~5.17]{li2018equilibrium}.

\begin{proposition}[Z.~Li~\cite{li2018equilibrium}]    \label{prop:pressures with respect to preimages}
	Let $f$ and $\phi$ satisfy the Assumptions in Section~\ref{sec:The Assumptions}. Then for each $x \in S^2$, we have
	\begin{equation}    \label{eq:pressures with respect to preimages}
 		P(f, \phi) = \lim_{n \to +\infty} \frac{1}{n} \log \!\sum_{y \in f^{-n}(x)}\!  \deg_{f^n}(y) \exp(S_n \phi(y)).
	\end{equation}
\end{proposition}

\begin{lemma}[Z.~Li \cite{li2018equilibrium}]    \label{lem:preimage_distortion_lemma}
    Let $f \: S^2 \mapping S^2$ be an expanding Thurston map and $\mathcal{C} \subseteq S^2$ be a Jordan curve containing $\post{f}$ with the property that $f^{n_{\mathcal{C}}}(\mathcal{C}) \subseteq \mathcal{C}$ for some $n_{\mathcal{C}} \in \n$. Let $d$ be a visual metric on $S^2$ for $f$ with expansion factor $\Lambda > 1$ and a linear local connectivity constant $L \geqslant 1$. Let $\phi \in C^{0,\holderexp}(S^2,d)$ be a real-valued \holder continuous function with an exponent $\holderexp \in (0,1]$. Then there exists a constant $C_2 = C_2(f, \mathcal{C}, d, \phi, \holderexp) \geqslant 1$ depending only on $f$, $\mathcal{C}$, $d$, $\phi$, and $\holderexp$ such that for each $x, \, y \in S^2$, and each $n \in \n_0$, we have
    \begin{equation}    \label{eq:preimage_distortion_lemma}
        \frac{  \sum\limits_{x' \in f^{-n}(x)} \deg_{f^{n}}(x') \exp(S_n \phi(x'))  }{  \sum\limits_{y' \in f^{-n}(y)} \deg_{f^{n}}(y') \exp(S_n \phi(y')) } \leqslant 
        \exp (4C_1 L d(x, y)^{\holderexp}) \leqslant C_2,
    \end{equation}
    where $C_1$ is the constant from Lemma~\ref{lem:distortion_lemma}. Quantitatively, we choose
    \begin{equation}    \label{eq:constant_C_2}
        C_2 \define \exp \Bigl(4C_1 L \bigl(\! \operatorname{diam}_{d}{\!(S^2)}\bigr)^{\holderexp} \Bigr) = \exp \left( 4 \frac{|\phi|_{\holderexp} C_0}{1 - \Lambda^{-\holderexp}} L\bigl(\!\diam{d}{S^2}\bigr)^{\holderexp} \right),
    \end{equation}
    where $C_0 > 1$ is the constant depending only on $f$, $\mathcal{C}$, and $d$ from Lemma~\ref{lem:basic_distortion}.
\end{lemma}

\begin{proof}[Proof of Proposition~\ref{prop:pressures with respect to tiles}]
	We fix a visual metric $d$ on $S^2$ for $f$. 

	Let integer $n \in \n$. We denote \[
	Z_{n}(f, \phi) \define \sum_{X^n \in \Tile{n}}\! \exp \!\bigl(\! \sup \bigl\{ S_n \phi(x) \describe x \in X^n \bigr\} \bigr).
	\]
	For each $X^n \in \Tile{n}$, we denote by $V(X^n)$ the set of $n$-vertices contained in $X^n$, i.e., $V(X^n) \define \{ x \in \Vertex{n} \describe x \in X^n \}$. Note that $\card{V(X^n)} = \card{\post{f}}$ since $X^n$ is a $\card{\post{f}}$-gon by Proposition~\ref{prop:properties cell decompositions}~\ref{item:prop:properties cell decompositions:tile is gon}. 

	By Lemma~\ref{lem:distortion_lemma}, for each $X^n \in \Tile{n}$ and each $v \in V(X^n)$, we have\[
	e^{S_n \phi(v)} \leqslant 
	\exp \!\bigl(\! \sup \bigl\{ S_n \phi(x) \describe x \in X^n \bigr\} \bigr) \leqslant 
	e^{ \Cdistortion } \, e^{S_n \phi(v)},
	\]
	so that\[
	\sum_{v \in V(X^n)} e^{S_n \phi(v)} \leqslant 
	\card{\post{f}} \exp \!\bigl(\! \sup \bigl\{ S_n \phi(x) \describe x \in X^n \bigr\} \bigr) \leqslant
	e^{ \Cdistortion } \sum_{v \in V(X^n)} e^{S_n \phi(v)}.
	\]
	Thus \[
	\sum_{X^n \in \Tile{n}} \sum_{v \in V(X^n)} e^{S_n \phi(v)} \leqslant 
	\card{\post{f}} Z_{n}(f, \phi) \leqslant
	e^{ \Cdistortion } \sum_{X^n \in \Tile{n}} \sum_{v \in V(X^n)} \, e^{S_n \phi(v)}.
	\]
	By Remark~\ref{rem:flower structure}, for each $n$-vertex $p \in \Vertex{n}$, there are exactly $2\deg_{f^n}(p)$ $n$-tiles containing $p$. Therefore,
	\begin{align*}
	\sum_{X^n \in \Tile{n}} \sum_{v \in V(X^n)} e^{S_n \phi(v)} 
		&= \sum_{p \in \Vertex{n}} 2\deg_{f^n}(p) e^{S_n \phi(p)}  \\
		&= \sum_{x \in \post{f}} \ \sum_{y \in f^{-n}(x)} 2\deg_{f^n}(y) e^{S_n \phi(y)},
	\end{align*}
	where the second inequality follows from the fact that $\Vertex{n} = f^{-n}(\post{f})$. Thus we deduce\[
	Z_{n}(f, \phi) \asymp \sum_{x \in \post{f}} \ \sum_{y \in f^{-n}(x)} \deg_{f^n}(y) e^{S_n \phi(y)},
	\]
	where the constant $C(\asymp)$ is independent of $n$. Moreover, applying Lemma~\ref{lem:preimage_distortion_lemma}, we have\[
	Z_{n}(f, \phi) \asymp \sum_{y \in f^{-n}(x_0)} \deg_{f^n}(y) e^{S_n \phi(y)}
	\]
	for some fixed $x_0 \in S^2$, where the constant $C(\asymp)$ is independent of $n$. Then \eqref{eq:pressures with respect to tiles} follows from Proposition~\ref{prop:pressures with respect to preimages}.
\end{proof}

The above arguments rely on the existence of $f$-invariant Gibbs measures with respect to $f$, $\mathcal{C}$, and $\phi$, which is proved in \cite[Theorem~5.16]{li2018equilibrium} via thermodynamic formalism. Actually, we can obtain the characterization of topological pressure \eqref{eq:pressures with respect to tiles} without using thermodynamic formalism when $f$ has no periodic critical points (see Proposition~\ref{prop:pressures with respect to tiles via cover}).

In the following proofs, we will use the definition of topological pressures formulated in \cite[Section~3.2]{przytycki2010conformal}, which is defined topologically via open covers and equivalent to the definitions via separated sets or Variational Principle (see \cite[Section~3]{przytycki2010conformal} for equivalence). For the convenience of the reader we record the definition briefly in the next paragraph.

Let $(X, d)$ be a compact metric space and let $T \: X \mapping X$ be a continuous transformation of $X$. Let $\varphi \: X \mapping \real$ be a continuous function. Let $\mathcal{U}$ be a finite open cover of $X$. For each integer $n \in \n$, we set \[
	\mathcal{U}^{n} \define \mathcal{U} \vee T^{-1}(\mathcal{U}) \vee \cdots \vee T^{-(n-1)}(\mathcal{U}),
\]
\begin{equation}    \label{eq:def of S_n set as sup}
	S_n \varphi(Y) = S_n^{T} \varphi(Y) \define \sup \left\{ \sum_{i=0}^{n-1} \varphi \circ T^{i}(x)  \describe  x \in Y\right\}
\end{equation}
for each set $Y \subseteq X$, and
\begin{equation}    \label{eq:partition function via cover}
	Z_n(T, \varphi, \mathcal{U}) \define \inf_{\mathcal{V}} \left\{ \sum_{V \in \mathcal{V}} \exp{S_n\varphi(V)} \right\},
\end{equation}
where $\mathcal{V}$ ranges over all covers of $X$ contained (in the sense of inclusion) in $\mathcal{U}^{n}$. Then the limit\[
	\lim_{n \to + \infty} \frac{1}{n} \log Z_n(T, \varphi, \mathcal{U})
\]
exists and is finite \cite[Lemma~3.2.1]{przytycki2010conformal}. Moreover, if $\{\mathcal{U}_m\}_{m \in \n}$ is a sequence of finite open covers of $X$ satisfying $\lim_{m \to +\infty} \diam{d}{\mathcal{U}_m} = 0$, then the following limit exists and is independent of the choice of such sequence \cite[Lemma~3.2.4]{przytycki2010conformal}, and we denote the limit by $P(T, \varphi)$:
\begin{equation}    \label{eq:def topological pressure by cover}
	P(T, \varphi) \define \lim_{m \to +\infty} \lim_{n \to + \infty} \frac{1}{n} \log Z_n(T, \varphi, \mathcal{U}_{m}).
\end{equation}
We call $P(T, \varphi)$ the \emph{topological pressure} of $T$ with respect to the \emph{potential} $\varphi$. One can see that the topological pressure $P(T, \varphi)$ defined above is independent of the metric $d$ since the convergence to zero of diameters of a sequence of subsets of $X$ does not depend on a compatible metric.

% proofs via the definition of pressures by coverings
\begin{proposition}    \label{prop:pressures with respect to tiles via cover}
	Let $f$, $\mathcal{C}$, and $\phi$ satisfy the Assumptions in Section~\ref{sec:The Assumptions}. If $f$ has no periodic critical points, then
	\begin{equation}    \label{eq:pressures with respect to tiles via cover}
 		P(f, \phi) = \lim_{n \to +\infty} \frac{1}{n} \log \!\sum_{X^n \in \mathbf{X}^{n}(f,\, \mathcal{C}) } \exp \!\bigl(\! \sup \bigl\{ S_n \phi(x) \describe x \in X^n \bigr\} \bigr).
	\end{equation}
\end{proposition}
\begin{proof}% another proof
	We fix a visual metric $d$ on $S^2$ for $f$. 

	Note that by Remark~\ref{rem:convergence of tile pressure for Thurston map} and \cite[Lemma~3.2.7]{przytycki2010conformal}, the limit in \eqref{eq:pressures with respect to tiles via cover} converges to a finite number and $P(f^{k}, \phi) = k P(f, \phi)$ for each $k \in \n$. Then, by Proposition~\ref{prop:properties cell decompositions}~\ref{item:prop:properties cell decompositions:iterate of cell decomposition}, it suffices to prove \eqref{eq:pressures with respect to tiles via cover} for $f^i$ for some $i \in \n$. Thus by Lemma~\ref{lem:invariant_Jordan_curve}, we can assume, without loss of generality, that there exists a Jordan curve $\mathcal{C} \subseteq S^2$ containing $\post{f}$ such that $f(\mathcal{C}) \subseteq \mathcal{C}$, and no $1$-tile joins opposite sides of $\mathcal{C}$.

	Indeed, Proposition~\ref{prop:characterization of pressures of subsystems in separated sets} shows that \[
		P(f, \phi) \leqslant \lim_{n \to +\infty} \frac{1}{n} \log \!\sum_{X^n \in \mathbf{X}^{n}(f,\, \mathcal{C}) } \exp S_n \phi(X^n)
	\]
	where $S_n\phi(X^n)$ is defined by \eqref{eq:def of S_n set as sup} (see \cite[Definition~20.2.1]{katok1995introduction}). In order to establish \eqref{eq:pressures with respect to tiles via cover}, it suffices to prove an inequality in the opposite direction, i.e.,
	\begin{equation}    \label{eq:greater inequality for pressures with respect to tiles via cover}
		P(f, \phi) \geqslant \lim_{n \to +\infty} \frac{1}{n} \log \!\sum_{X^n \in \mathbf{X}^{n}(f,\, \mathcal{C}) } \exp S_n \phi(X^n).
	\end{equation}
	For each integer $m \in \n$, the set of all $m$-flowers $\Flower{m}$ defined in \eqref{eq:set_of_n-flowers} is a finite open cover of $S^2$. By Lemma~\ref{lem:visual_metric}~\ref{item:lem:visual_metric:diameter of cell}, we have $\lim_{m \to +\infty} \diam{d}{\Flower{m}} = 0$. Then it follows from the definition of topological pressure (see~\eqref{eq:def topological pressure by cover}) that\[
		P(f, \phi) = \lim_{m \to +\infty}  \lim_{n \to + \infty} \frac{1}{n} \log Z_n(f, \phi, \Flower{m}).
	\]

	Fix arbitrary integers $m, n \in \n$. Let $\mathcal{U}_{m} \define \Flower{m}$ and $\mathcal{V}$ be an arbitrary cover of $S^2$ contained (in the sense of inclusion) in $\mathcal{U}_{m}^{n}$, where\[
		\mathcal{U}_{m}^{n} \define \mathcal{U}_{m} \vee f^{-1}(\mathcal{U}_{m}) \vee \cdots \vee f^{-(n-1)}(\mathcal{U}_{m}).
	\]
	Then for each $V \in \mathcal{V}$, we can write
	\begin{equation}    \label{eq:expression for V}
		V = \bigcap_{i = 0}^{n-1} f^{-i}(\flower{m}{p_i})
	\end{equation}
	for some $p_i \in \Vertex{m}$ for $i \in \{0, \, 1, \, \dots, \, n-1\}$. Applying \cite[Lemma~5.8]{li2015weak} (note that we assume that $f(\mathcal{C}) \subseteq \mathcal{C}$), we have
	\begin{equation}    \label{eq:V cover by flower}
		V \subseteq V' \define \bigcup_{x \in E_m(p_0, p_1, \dots, p_{n-2}; p_{n-1})} \flower{m + n - 1}{x},
	\end{equation}
	where $E_m$ is defined as: for $m \in \n_0$, $n \in \n$, $q \in S^2$, and $q_i \in \Vertex{m}$ for $i \in \{0, \, 1, \, \dots, \, n-1\}$,
	\begin{equation}    \label{eq:definition of E_m}
		E_m(q_0, q_1, \dots, q_{n-1}; q) \define \bigl\{ x \in f^{-n}(q) \describe f^{i}(x) \in \cflower{m}{q_i},\, i \in \{0, \, 1, \, \dots, \, n-1\} \bigr\}.
	\end{equation}
	Note that $V'$ is determined by $V$ via \eqref{eq:expression for V} and \eqref{eq:V cover by flower}. One sees that $V$ relates to $V'$ by \eqref{eq:V cover by flower}, where $V'$ is a union of some flowers so that one can use combinatorial structures and estimates of tiles.

	We next estimate the oscillation of $S_n\phi$ on $V'$ to obtain an upper bound for the difference between $S_n\phi(V)$ and $S_n\phi(V')$. To keep the notation simple, we denote $E_m(V) = E_m(p_0, p_1, \dots, p_{n-2}; p_{n-1})$. Indeed, $E_m(V)$ is determined by $V$ via \eqref{eq:expression for V} and \eqref{eq:V cover by flower}.

	Noting that $f^{i}(E_m(V)) \subseteq \cflower{m}{p_i}$ for $i \in \{0, \, 1, \, \dots, \, n-1\}$ by \eqref{eq:definition of E_m}, it follows from Lemma~\ref{lem:visual_metric}~\ref{item:lem:visual_metric:diameter of cell} that
	\begin{equation}    \label{eq:diam f^i E_m}
		\diam{d}{f^{i}(E_m(V))} \leqslant \diam{d}{\cflower{m}{p_i}} \leqslant  2C \Lambda^{-m}\quad \text{for } i \in \{0, \, 1, \, \dots, \, n-1\},
	\end{equation}
	where $\Lambda > 1$ is the expansion factor of $d$ and $C \geqslant 1$ is the constant depending only on $f$, $\mathcal{C}$, and $d$ from Lemma~\ref{lem:visual_metric}. 

	Now let $x', y' \in V'$  be arbitrary. By the definition of $V'$, there exist $x, \, y \in E_m(V)$ such that $x' \in \flower{m + n - 1}{x}$ and $y' \in \flower{m + n - 1}{y}$. Since $E_m(V) \subseteq f^{-n+1}(p_{n-1}) \subseteq \Vertex{m + n - 1}$, by Remark~\ref{rem:flower preserve under iterate}, we have\[
		f^{i}(x') \in f^{i}(\flower{m + n - 1}{x}) = \flower{m + n - 1 - i}{f^{i}(x)} 
	\]
	for each $i \in \{0, \, 1, \, \dots, \, n-1\}$, and similarly, the corresponding results hold for $y'$. Thus by Remark~\ref{rem:flower structure}, Lemma~\ref{lem:visual_metric}~\ref{item:lem:visual_metric:diameter of cell}, and \eqref{eq:diam f^i E_m},
	\begin{align*}
	d(f^{i}(x'), f^{i}(y')) &\leqslant d(f^{i}(x), f^{i}(y)) + d(f^{i}(x'), f^{i}(x)) + d(f^{i}(y'), f^{i}(y)) \\
		&\leqslant \diam{d}{f^{i}(E_m(V))} + 2C\Lambda^{-m}  \\
		&\leqslant 4C\Lambda^{-m}
	\end{align*}
	for each $i \in \{0, \, 1, \, \dots, \, n-1\}$. This together with our assumption that $\phi \in C^{0,\holderexp}(S^2,d)$ is \holder continuous with an exponent $\holderexp \in (0,1]$ implies
	\begin{align*}
	|S_n\phi(x') - S_n\phi(y')| &\leqslant \sum_{i=0}^{n-1} |\phi(f^{i}(x')) -\phi(f^{i}(y'))|  \\
		&\leqslant \sum_{i=0}^{n-1} |\phi|_{\holderexp}  (d(f^{i}(x'), f^{i}(y')))^{\holderexp}  \\
		&\leqslant \sum_{i=0}^{n-1} |\phi|_{\holderexp}  ( 4C\Lambda^{-m} )^{\holderexp}  \\
		&\leqslant 4C |\phi|_{\holderexp} \Lambda^{-\holderexp m} n \\ 
		&= \operatorname{osc}(m)n
	\end{align*}
	for each $x', y' \in V'$, where we write $\operatorname{osc}(m) \define 4C |\phi|_{\holderexp} \Lambda^{-\holderexp m}$ for simplicity. Therefore, we obtain
	\begin{equation}    \label{eq:estimate for potential}
		|S_n \phi(V') - S_n \phi(V)| \leqslant \operatorname{osc}(m)n.
	\end{equation}
	One can see that $\operatorname{osc}(m)$ depends only on $f$, $\mathcal{C}$, $d$, $\phi$, and $m$. Moreover,
	\begin{equation}    \label{eq:osc m tend to 0}
		\lim_{m \to +\infty} \operatorname{osc}(m) = 0.
	\end{equation}

	Besides the estimate~\eqref{eq:estimate for potential}, to obtain \eqref{eq:greater inequality for pressures with respect to tiles via cover}, we need two extra combinatorial bounds~\eqref{eq:bound for local degree} and \eqref{eq:bound for card E_m}. We emphasize that these two estimates rely on the assumption that $f$ has no periodic critical points.

	Under our assumption that $f$ has no periodic critical points, there exists a constant $N \in \n$ such that
	\begin{equation}    \label{eq:bound for local degree}
		\deg_{f^{k}}(x) \leqslant N
	\end{equation}
	for all $x \in S^2$ and all $k \in \n$ (\cite[Lemma~18.6]{bonk2017expanding}). 

	Again under the same assumption, \cite{li2015weak} proves an upper bound for $\card{E_m(V)}$ (see \cite[Theorem~5.10]{li2015weak}). Briefly speaking, there exists a function $D \: \n \times \n \mapping (0, +\infty)$ depending only on $f$, $\mathcal{C}$, and $d$ such that
	\begin{equation}    \label{eq:bound for card E_m}
		\sup_{V \in \mathcal{V}} \card{E_m(V)} \leqslant e^{nD(m,n)},
	\end{equation}
	and the function $D(m,n)$ satisfies
	\begin{equation}    \label{eq:property of function D}
		\lim_{m \to +\infty} \lim_{n \to +\infty} D(m,n) = 0.
	\end{equation}
	We will not give the explicit formula for function $D(m,n)$ here, because it is somewhat technical and \eqref{eq:property of function D} is enough for our proof.
	\begin{comment}
	\[
		\sup_{V \in \mathcal{V}} \card{E_m(V)} \leqslant (\deg f)^{N_c(\frac{n}{M_m}) + 1}
	\]

	\[
		N_c = \max\left\{ \min\left\{ i \in \n \describe f^{j}(x) \notin \crit{f} \text{ if } j \geqslant i \right\} \describe x \in \crit{f} \right\}
	\]

	\[
		M_i = \left\lfloor \log_{K}\left(  \frac{D_{c} - \tau(3C\Lambda^{-i})}{\tau(3C\Lambda^{-i})}\right) \right\rfloor - 2.
	\]
	\end{comment}

	Combining \eqref{eq:bound for card E_m} and \eqref{eq:bound for local degree}, we obtain
	\begin{align*}
	\exp{S_n\phi(V')} &= \exp{S_n\phi(\overline{V'})} \\
		&\geqslant \sum_{x \in E_m(V)} \frac{ \exp{S_n\phi(\cflower{m + n - 1}{x})} }{ e^{nD(m,n)} } \\
		&\geqslant \sum_{x \in E_m(V)} \sum_{ \substack{X^{m+n-1} \subseteq \cflower{m+n-1}{x} \\ X^{m+n-1} \in \tile{m + n - 1}} } \frac{ \exp{S_n\phi(X^{m+n-1})} }{ 2N e^{nD(m,n)} } \\
		&\geqslant \sum_{ \substack{ X^{m + n - 1} \in \tile{m + n - 1} \\ X^{m + n - 1} \subseteq \overline{V'} } } \frac{ \exp{S_n\phi(X^{m+n-1})} }{ 2N e^{nD(m,n)} }
	\end{align*}
	for each $V \in \mathcal{V}$, where the second inequality follows from Remark~\ref{rem:flower structure} and the last inequality follows from \eqref{eq:V cover by flower}.	Since $\{V' \describe V \in \mathcal{V}\}$ is an open cover of $S^2$, we have\[
		\bigcup \tile{m+n-1} = \bigcup_{V \in \mathcal{V}} \overline{V'} =  
		\bigcup_{V \in \mathcal{V}} \bigcup_{\substack{ X^{m + n - 1} \in \tile{m + n - 1} \\ X^{m + n - 1} \subseteq \overline{V'} } } X^{m + n -1}.
	\]
	Thus
	\begin{align*}
	\sum_{V \in \mathcal{V}} \exp{S_n\phi(V')} 
		&\geqslant \sum_{X^{m+n-1} \in \tile{m+n-1} } \frac{\exp{S_n\phi(X^{m+n-1})}}{ 2N e^{nD(m,n)} }  \\
		&\geqslant \sum_{X^{m+n-1} \in \tile{m+n-1} } \frac{\exp{S_{m+n-1}\phi(X^{m+n-1})}}{ 2N e^{m\uniformnorm{\phi}} e^{nD(m,n)} }.
	\end{align*}
	Combining this with \eqref{eq:estimate for potential}, we get
	\begin{align*}
	P(f, \phi) &= \lim_{m \to +\infty} \lim_{n \to +\infty} \frac{1}{n} \log \inf_{\mathcal{V}} \left\{ \sum_{V \in \mathcal{V}} \exp{S_n\phi(V)} \right\} \\
		&\geqslant \lim_{m \to +\infty} \lim_{n \to +\infty} \frac{1}{n} \log \inf_{\mathcal{V}} \left\{ e^{-\operatorname{osc}(m)n} \sum_{V \in \mathcal{V}} \exp{S_n\phi(V')} \right\} \\
		&\geqslant \lim_{m \to +\infty} \lim_{n \to +\infty} \frac{1}{n} \log \sum_{X^{m+n-1} \in \tile{m+n-1} } 
				\frac{ \exp{S_{m+n-1}\phi(X^{m+n-1})} }{ 2N e^{m\uniformnorm{\phi}} e^{nD(m,n)} e^{\operatorname{osc}(m)n} } \\
		&= \lim_{m \to +\infty} \lim_{n \to +\infty} \frac{1}{n} \log \sum_{X^{m+n-1} \in \tile{m+n-1} } \exp{S_{m+n-1}\phi(X^{m+n-1})} \\
		&= \lim_{n \to +\infty} \frac{1}{n} \log \!\sum_{X^n \in \tile{n} } \exp S_n \phi(X^n),
	\end{align*}
	where the last but one equality follows from \eqref{eq:osc m tend to 0} and \eqref{eq:property of function D}, and the last equality follows from the fact that the limit in \eqref{eq:pressures with respect to tiles via cover} exists. Therefore \eqref{eq:greater inequality for pressures with respect to tiles via cover} holds.
\end{proof}

% proofs via the definition of pressures by separated sets

\begin{proposition}    \label{prop:subsystem pressures with respect to tiles via cover}
Let $f$, $\mathcal{C}$, and $\phi$ satisfy the Assumptions in Section~\ref{sec:The Assumptions}. We assume in addition that $f(\mathcal{C}) \subseteq \mathcal{C}$ and $f$ has no periodic critical points. Consider $F \in \subsystem$. If the map $F$ is not degenerate, then
\begin{equation}    \label{eq:subsystem pressures with respect to tiles via cover}
	P(F|_{\limitset}, \phi) = \lim_{n \to +\infty} \frac{1}{n} \log \!\sum_{X^n \in \Domain{n}} \exp \!\bigl(\! \sup \bigl\{ S_n^{F} \phi(x) \describe x \in X^n \bigr\} \bigr).
\end{equation}
\end{proposition}
\begin{proof}
	We fix a visual metric $d$ on $S^2$ for $f$. For convenience we set $\widehat{F} \define F|_{\limitset} = f|_{\limitset}$ and $\limitset^n $ for each $n \in \n_0$.

	Note that Proposition~\ref{prop:characterization of pressures of subsystems in separated sets} shows that\[
		\fpressure \leqslant \lim_{n \to +\infty} \frac{1}{n}\log \sum_{X^n \in \Domain{n}} \exp{S_n^{F} \phi(X^n)},
	\]
	where $S_n^{F} \phi(X^n)$ is defined by \eqref{eq:def of S_n set as sup}. In order to establish \eqref{eq:subsystem pressures with respect to tiles via cover}, it suffices to prove an inequality in the opposite direction, i.e.,
	\begin{equation}    \label{eq:greater inequality for subsystem pressures with respect to tiles via cover}
		\fpressure \geqslant \lim_{n \to +\infty} \frac{1}{n}\log \sum_{X^n \in \Domain{n}} \exp{S_n^{F} \phi(X^n)}.
	\end{equation}
	For each integer $m \in \n$, the set of all $m$-flowers $\Flower{m}$ defined in \eqref{eq:set_of_n-flowers} is a finite open cover of $S^2$. Thus, for each $m \in \n$, the set
	\begin{equation}    \label{eq:def limitset flower cover}
		\mathbf{\widehat{W}}^{m} \define \{ W^{m} \cap \limitset \describe W^m \in \Flower{m} \}
	\end{equation}
	is a finite open cover of $\limitset$. Hence, by Lemma~\ref{lem:visual_metric}, we have $\lim_{m \to +\infty} \diam{d}{\mathbf{\widehat{W}}^{m}} = 0$. Then it follows from the definition of topological pressure (see~\eqref{eq:def topological pressure by cover}) that\[
		\fpressure = \lim_{m \to +\infty}  \lim_{n \to + \infty} \frac{1}{n} \log Z_n(\widehat{F}, \phi, \mathbf{\widehat{W}}^{m}).
	\]

	Fix arbitrary integers $m,\, n \in \n$. Let $\mathcal{\widehat{U}}_{m} = \mathbf{\widehat{W}}^{m}$ and $\mathcal{\widehat{V}}$ be an arbitrary cover of $\limitset$ contained (in the sense of inclusion) in $\mathcal{\widehat{U}}_{m}^{n}$, where\[
		\mathcal{\widehat{U}}_{m}^{n} \define \mathcal{\widehat{U}}_{m} \vee \widehat{F}^{-1}(\mathcal{\widehat{U}}_{m}) \vee \cdots \vee \widehat{F}^{-(n-1)}(\mathcal{\widehat{U}}_{m}).
	\]
	Then for each $\widehat{V} \in \mathcal{\widehat{V}}$, we can write
	\begin{equation}    \label{eq:expression for subsystem V}
		\widehat{V} = \bigcap_{i = 0}^{n-1} \widehat{F}^{-i} \bigl(W^{m}(p_i)\cap \limitset \bigr)
	\end{equation}
	for some $p_i \in \Vertex{m}$ for $i \in \{0, \, 1, \, \dots, \, n-1\}$. Noting that \[
		\widehat{V} \subseteq \bigcap_{i = 0}^{n-1} f^{-i} \bigl(W^{m}(p_i)\cap \limitset \bigr) \subseteq \bigcap_{i = 0}^{n-1} f^{-i}(W^{m}(p_i)),
	\]
	it follows from \cite[Lemma~5.8]{li2015weak} (note that we assume that $f(\mathcal{C}) \subseteq \mathcal{C}$) that
	\begin{equation}    \label{eq:subsystem V cover by V'}
		\widehat{V} \subseteq V' \define \bigcup_{x \in E_m(p_0, p_1, \dots, p_{n-2}; p_{n-1})} \flower{m + n - 1}{x},
	\end{equation}
	where $E_m$ is defined as: for $m \in \n_0$, $n \in \n$, $q \in S^2$, and $q_i \in \Vertex{m}$ for $i \in \{0, \, 1, \, \dots, \, n-1\}$,
	\begin{equation}    \label{eq:subsystem:definition of E_m}
		E_m(q_0, q_1, \dots, q_{n-1}; q) \define \bigl\{ x \in f^{-n}(q) \describe f^{i}(x) \in \cflower{m}{q_i},\, i \in \{0, \, 1, \, \dots, \, n-1\} \bigr\}.
	\end{equation}
	Moreover, we denote by $V''$ the $(m + n -1)$-bouquet of $\overline{V'}$ (see \eqref{eq:Un bouquet of set}), i.e.,
	\begin{equation}    \label{eq:def V''}
		V'' \define U^{m + n - 1}\bigl( \overline{V'} \bigr) = \bigcup_{x \in \overline{V'}} U^{m + n - 1}(x).
	\end{equation}
	
	Note that $V'$ and $V''$ are determined by $\widehat{V}$ via \eqref{eq:expression for subsystem V} and \eqref{eq:subsystem V cover by V'}. one sees that $\widehat{V}$ relates to $V'$ and $V''$ by \eqref{eq:subsystem V cover by V'} and \eqref{eq:def V''}, where $V'$ is a union of some $(m + n - 1)$-flowers and $V''$ is a union of some $(m + n - 1)$-tiles. Therefore, we can use combinatorial structures and estimates of tiles.

	We next estimate the oscillation of $S_n \phi$ on $V''$ to obtain an upper bound for the difference between $S_n^{\widehat{F}}\phi(\widehat{V})$ and $S_n\phi(V'')$. To keep the notation simple, we denote by $E_m(\widehat{V})$ the set $E_m(p_0, p_1, \dots, p_{n-2}; p_{n-1})$ since the set $E_m(\widehat{V})$ is determined by $\widehat{V}$ via \eqref{eq:expression for subsystem V} and \eqref{eq:subsystem V cover by V'}.

	Noting that $f^{i}(E_m(\widehat{V})) \subseteq \cflower{m}{p_i}$ for $i \in \{0, \, 1, \, \dots, \, n-1\}$ by \eqref{eq:subsystem:definition of E_m}, it follows from Lemma~\ref{lem:visual_metric}~\ref{item:lem:visual_metric:diameter of cell} that
	\begin{equation}    \label{eq:diam f^i E_m subsystem V}
		\diam{d}{f^{i}(E_m(V))} \leqslant \diam{d}{\cflower{m}{p_i}} \leqslant  2C \Lambda^{-m}\quad \text{for } i \in \{0, \, 1, \, \dots, \, n-1\},
	\end{equation}
	where $\Lambda > 1$ is the expansion factor of $d$ and $C \geqslant 1$ is the constant depending only on $f$, $\mathcal{C}$, and $d$ from Lemma~\ref{lem:visual_metric}. 

	Now let $x'', y'' \in V''$  be arbitrary. By the definition of $V''$ (recall \eqref{eq:def V''}), there exist $x', y' \in \overline{V'}$ such that $x'' \in U^{m + n - 1}(x')$ and $y'' \in U^{m + n - 1}(y')$. By \eqref{eq:bouquet preserve under iterate}, we have\[
		f^{i}(x'') \in f^{i}(U^{m + n - 1}(x')) = U^{m + n - 1 - i}(f^{i}(x')) 	
	\] 
	for each $i \in \{0, \, 1, \, \dots, \, n-1\}$, and similarly, the corresponding results hold for $y''$. Thus by Lemma~\ref{lem:visual_metric}~\ref{item:lem:visual_metric:bouquet bounded by ball},
	\begin{align*}
		d(f^{i}(x''), f^{i}(y'')) &\leqslant d(f^{i}(x''), f^{i}(x')) + d(f^{i}(y''), f^{i}(y')) + d(f^{i}(x'), f^{i}(y')) \\
		&\leqslant 2K \Lambda^{-(m + n - 1 - i)} + d(f^{i}(x'), f^{i}(y'))  \\
		&\leqslant 2K \Lambda^{-m} + d(f^{i}(x'), f^{i}(y')) 
	\end{align*}
	for each $i \in \{0, \, 1, \, \dots, \, n-1\}$, where $K \geqslant 1$ is the constant depending only on $f$, $\mathcal{C}$, and $d$ from Lemma~\ref{lem:visual_metric}. 
	
	We next estimate $d(f^{i}(x'), f^{i}(y'))$. Since $x', y' \in \overline{V'}$, by the definition of $V'$ (see \eqref{eq:subsystem V cover by V'}), there exist $x, \, y \in E_m(\widehat{V})$ such that $x' \in \cflower{m + n - 1}{x}$ and $y' \in \cflower{m + n - 1}{y}$. Noting that $E_m(\widehat{V}) \subseteq f^{-n+1}(p_{n-1}) \subseteq \Vertex{m + n - 1}$, by Remark~\ref{rem:flower preserve under iterate}, we have\[
		f^{i}(x') \in f^{i}(\flower{m + n - 1}{x}) = \flower{m + n - 1 - i}{f^{i}(x)} 
	\]
	for each $i \in \{0, \, 1, \, \dots, \, n-1\}$, and similarly, the corresponding results hold for $y'$. Thus by Remark~\ref{rem:flower structure}, Lemma~\ref{lem:visual_metric}~\ref{item:lem:visual_metric:diameter of cell}, and \eqref{eq:diam f^i E_m subsystem V},
	\begin{align*}
	d(f^{i}(x'), f^{i}(y')) &\leqslant d(f^{i}(x), f^{i}(y)) + d(f^{i}(x'), f^{i}(x)) + d(f^{i}(y'), f^{i}(y)) \\
		&\leqslant \diam{d}{f^{i}(E_m(V))} + 2C\Lambda^{-m}  \\
		&\leqslant 4C\Lambda^{-m}
	\end{align*}
	for each $i \in \{0, \, 1, \, \dots, \, n-1\}$. This together with our assumption that $\phi \in C^{0,\holderexp}(S^2,d)$ is \holder continuous with an exponent $\holderexp \in (0,1]$ implies
	\begin{align*}
	|S_n\phi(x'') - S_n\phi(y'')| &\leqslant \sum_{i=0}^{n-1} |\phi(f^{i}(x'')) -\phi(f^{i}(y''))|  \\
		&\leqslant \sum_{i=0}^{n-1} |\phi|_{\holderexp}  \bigl(d(f^{i}(x''), f^{i}(y'')) \bigr)^{\holderexp}  \\
		&\leqslant \sum_{i=0}^{n-1} |\phi|_{\holderexp}  \bigl( (2K + 4C) \Lambda^{-m} \bigr)^{\holderexp}  \\
		&\leqslant (2K + 4C) |\phi|_{\holderexp} \Lambda^{-\holderexp m} n \\ 
		&= \operatorname{osc}(m)n
	\end{align*}
	for each $x'', y'' \in V''$, where we denote by $\operatorname{osc}(m)$ the quantity $(2K + 4C) |\phi|_{\holderexp} \Lambda^{-\holderexp m}$ for simplicity. Since $\widehat{V} \subseteq V' \subseteq V''$ and $S_n^{\widehat{F}}\phi = S_n\phi$ on $\widehat{V}$, we obtain
	\begin{equation}    \label{eq:subsystem:estimate for potential}
		|S_n \phi(V'') - S_n^{\widehat{F}} \phi(\widehat{V})| \leqslant \operatorname{osc}(m)n.
	\end{equation}
	One can see that $\operatorname{osc}(m)$ depends only on $f$, $\mathcal{C}$, $d$, $\phi$, and $m$. Moreover,
	\begin{equation}    \label{eq:subsystem:osc m tend to 0}
		\lim_{m \to +\infty} \operatorname{osc}(m) = 0.
	\end{equation}

	Besides the estimate~\eqref{eq:subsystem:estimate for potential}, to obtain \eqref{eq:greater inequality for subsystem pressures with respect to tiles via cover}, we need three extra combinatorial bounds~\eqref{eq:subsystem:bound for local degree}, \eqref{eq:upper bound for bouquet of tile}, and \eqref{eq:subsystem:bound for card E_m}. We emphasize that these two estimates rely on the assumption that $f$ has no periodic critical points.

	Under our assumption that $f$ has no periodic critical points, there exists a constant $N \in \n$ depending only on $f$ such that
	\begin{equation}    \label{eq:subsystem:bound for local degree}
		\deg_{f^{k}}(x) \leqslant N
	\end{equation}
	for all $x \in S^2$ and all $k \in \n$ (\cite[Lemma~18.6]{bonk2017expanding}). 

	Under the same assumption, there exists a constant $N' \in \n$ depending only on $f$ such that for each $k \in \n$ and each $k$-tile $X^k \in \Tile{k}$, the set $U^{k}(X^k)$ is a union of at most $N'$ distinct $k$-tiles, i.e.,
	\begin{equation}    \label{eq:upper bound for bouquet of tile}
		\operatorname{card}{\! \bigl\{Y^k \in \tile{k} \describe \text{there exists an } k\text{-tile } Z^k \in \tile{k} \text{ with } Z^k \cap X^k \ne \emptyset \text{ and } Z^k \cap Y^k \ne \emptyset \bigr\}} \leqslant N'.
	\end{equation}
	Indeed, since each $k$-flower $W^{k}(q)$ for $q \in \vertex{k}$ is covered by exactly $2 \deg_{f^{k}}(q)$ distinct $k$-tiles (recall Remark~\ref{rem:flower structure}), for each $x \in S^2$, $U^{k}(x)$ is covered by a bounded number of $k$-flowers and thus covered by a bounded number, independent of $x \in S^2$ and $k \in \n_0$, of distinct $k$-tiles. Moreover, noting that $X^k$ is an $\card{\post{f}}$-gon (recall Proposition~\ref{prop:properties cell decompositions}~\ref{item:prop:properties cell decompositions:tile is gon}) and $U^{k}(X^k)$ coincides with the $k$-bouquet of the set of $k$-vertices in $X^k$, the set $U^{k}(X^k)$ is covered by a bounded number of distinct $k$-tiles.

	Again under the same assumption, \cite{li2015weak} proves an upper bound for $\card{E_m(\widehat{V})}$ (see \cite[Theorem~5.10]{li2015weak}). Briefly speaking, there exists a function $D \: \n \times \n \mapping (0, +\infty)$ depending only on $f$, $\mathcal{C}$, and $d$ such that
	\begin{equation}    \label{eq:subsystem:bound for card E_m}
		\sup_{\widehat{V} \in \mathcal{\widehat{V}}} \card{E_m(\widehat{V})} \leqslant e^{n D(m,n)},
	\end{equation}
	and the function $D(m,n)$ satisfies
	\begin{equation}    \label{eq:subsystem:property of function D}
		\lim_{m \to +\infty} \lim_{n \to +\infty} D(m,n) = 0.
	\end{equation}
	We will not give the explicit formula for function $D(m,n)$ here, because it is somewhat technical and \eqref{eq:subsystem:property of function D} is enough for our proof.

	By \eqref{eq:subsystem V cover by V'}, \eqref{eq:def V''}, and the definition of bouquets of sets (see \eqref{eq:Un bouquet of set}), we can write $V''$ as
	\begin{align}
	V'' &= \bigcup_{x \in E(\widehat{V})} U^{m + n - 1} \bigl( \cflower{m+n-1}{x} \bigr) \nonumber \\
		&= \bigcup_{x \in E(\widehat{V})}   \bigcup_{\substack{ Y^{m + n - 1} \subseteq \cflower{m+n-1}{x} \\ Y^{m + n - 1} \in \tile{m + n - 1}}} U^{m + n - 1}(Y^{m + n - 1})  \nonumber\\
		&= \bigcup_{x \in E(\widehat{V})}   \bigcup_{\substack{ Y^{m + n - 1} \subseteq \cflower{m+n-1}{x} \\ Y^{m + n - 1} \in \tile{m + n - 1}}}    \bigcup_{ \substack{ X^{m + n - 1} \subseteq U^{m + n - 1}(Y^{m + n - 1}) \\ X^{m + n - 1} \in \tile{m + n - 1} } }  X^{m + n - 1}.     \label{eq:V'' union of tile}
	\end{align}
	Combining \eqref{eq:subsystem:bound for card E_m}, \eqref{eq:subsystem:bound for local degree}, and \eqref{eq:upper bound for bouquet of tile}, we obtain
	\begin{align*}
	\exp{S_n\phi(V'')} 
		&\geqslant \sum_{x \in E_m(\widehat{V})} \frac{ \exp{S_n\phi \bigl( U^{m + n - 1} \bigl( \cflower{m+n-1}{x} \bigr) \bigr)} }{ e^{nD(m,n)} } \\
		&\geqslant \sum_{x \in E_m(\widehat{V})} 	\sum_{ \substack{ Y^{m+n-1} \subseteq \cflower{m+n-1}{x} \\ Y^{m+n-1} \in \tile{m + n - 1}} } \frac{ \exp{S_n\phi( U^{m + n - 1}(Y^{m + n - 1}) )} }{ 2N e^{nD(m,n)} } \\
		&\geqslant \sum_{x \in E_m(\widehat{V})}	\sum_{ \substack{ Y^{m+n-1} \subseteq \cflower{m+n-1}{x} \\ Y^{m+n-1} \in \tile{m + n - 1}} }    \sum_{ \substack{ X^{m + n - 1} \subseteq U^{m + n - 1}(Y^{m + n - 1}) \\ X^{m + n - 1} \in \tile{m + n - 1} } }	\frac{ \exp{S_n\phi( X^{m + n - 1} )} }{ 2N N' e^{nD(m,n)} } \\
		&\geqslant \sum_{ \substack{ X^{m + n - 1} \subseteq V'' \\ X^{m + n - 1} \in \tile{m + n - 1} } }     \frac{ \exp{S_n\phi(X^{m+n-1})} }{ 2N N' e^{nD(m,n)} }
	\end{align*}
	for each $\widehat{V} \in \mathcal{\widehat{V}}$, where the second inequality follows from Remark~\ref{rem:flower structure} and the last inequality follows from \eqref{eq:V'' union of tile}.	

	Note that the map $F$ is not degenerate by our assumptions. Then it follows from Proposition~\ref{prop:no degenerate no die} that \[
		\bigcup \Domain{m + n - 1} \subseteq U^{m + n - 1}(\limitset).
	\]	  
	Since $\mathcal{\widehat{V}}$ is an open cover of $\limitset$ and $\widehat{V} \subseteq V' \subseteq V''$ for each $\widehat{V} \in \mathcal{\widehat{V}}$ (here $V'$ and $V''$ are determined by $\widehat{V}$ via \eqref{eq:expression for subsystem V} and \eqref{eq:subsystem V cover by V'}), we have\[
		\bigcup \Domain{m + n - 1} \subseteq 
		\bigcup_{\widehat{V} \in \mathcal{\widehat{V}}} V'' =  
		\bigcup_{\widehat{V} \in \mathcal{\widehat{V}}} \bigcup_{\substack{ X^{m + n - 1} \subseteq V'' \\ X^{m + n - 1} \in \tile{m + n - 1} } } X^{m + n -1}.
	\]
	Thus
	\begin{align*}
	\sum_{\widehat{V} \in \mathcal{\widehat{V}}} \exp{S_n\phi(V'')} 
		&\geqslant \sum_{X^{m+n-1} \in \Domain{m+n-1} } \frac{\exp{S_n\phi(X^{m+n-1})}}{ 2N N' e^{nD(m,n)} }  \\
		&\geqslant \sum_{X^{m+n-1} \in \Domain{m+n-1} } \frac{\exp{S_{m+n-1}\phi(X^{m+n-1})}}{ 2N N' e^{m\uniformnorm{\phi}} e^{nD(m,n)} }.
	\end{align*}
	Combining this with \eqref{eq:estimate for potential}, we get
	\begin{align*}
		\fpressure &= \lim_{m \to +\infty} \lim_{n \to +\infty} \frac{1}{n} \log \inf_{\mathcal{\widehat{V}}} \left\{ \sum_{\widehat{V} \in \mathcal{\widehat{V}}} \exp{S_n^{\widehat{F}}\phi(\widehat{V})} \right\} \\
		&\geqslant \lim_{m \to +\infty} \lim_{n \to +\infty} \frac{1}{n} \log \inf_{\mathcal{\widehat{V}}} \left\{ e^{-\operatorname{osc}(m)n} \sum_{\widehat{V} \in \mathcal{\widehat{V}}} \exp{S_n \phi(V'')} \right\} \\
		&\geqslant \lim_{m \to +\infty} \lim_{n \to +\infty} \frac{1}{n} \log \sum_{X^{m+n-1} \in \Domain{m+n-1} } 
				\frac{ \exp{S_{m+n-1}\phi(X^{m+n-1})} }{ 2N N' e^{m\uniformnorm{\phi}} e^{nD(m,n)} e^{\operatorname{osc}(m)n} } \\
		&= \lim_{m \to +\infty} \lim_{n \to +\infty} \frac{1}{n} \log \sum_{X^{m+n-1} \in \Domain{m+n-1} } \exp{S_{m+n-1}\phi(X^{m+n-1})} \\
		&= \lim_{n \to +\infty} \frac{1}{n} \log \!\sum_{X^n \in \Domain{n} } \exp S_n^{F} \phi(X^n),
	\end{align*}
	where the last but one equality follows from \eqref{eq:subsystem:osc m tend to 0} and \eqref{eq:subsystem:property of function D}, and the last equality holds since the limit in \eqref{eq:subsystem pressures with respect to tiles via cover} exists. Therefore \eqref{eq:greater inequality for subsystem pressures with respect to tiles via cover} holds.
\end{proof}

\begin{comment}
\sum_{X^n \in \mathbf{X}^{n}(f,\, \mathcal{C}) } \sup_{x \in X^n} e^{S_n \phi(x)}.

Let $f \: S^2 \mapping S^2$ be an expanding Thurston map with a Jordan curve $\mathcal{C}\subseteq S^2$ satisfying $\post{f} \subseteq \mathcal{C}$. 
\end{comment}
